# Supplementary material for: Semantic 3D Reconstruction with Finite Element Bases
Source: arXiv:1710.01749 source file (2017-10-04)
Supplement: Supplementary file 7 [file proofsc.tex]

\subsection{Gradient in Lagrange basis}\label{sec:gradient_lagrange}
short proof as in why is it like this. have already

\subsection{Continuous vs Discrete}
\label{sec:continuous_discrete_discussion}

\subsection{optimization - dykstra}
\label{sec:data_cost}

\subsection{grid vs fem}
\label{sec:GridvsFEM}

\subsection{Adaptiveness}
\label{sec:adaptiveness}

\subsection{Data cost integration}
\label{sec:data_cost}
