# Supplementary material for: Semantic 3D Reconstruction with Finite Element Bases
Source: arXiv:1710.01749 source file (2017-10-04)
Supplement: Supplementary file 9 [file suppContinuous.tex]

%
\subsection{Non-Metricness: Continuous vs. Discrete}
%
\begin{comment}
Although we finally desire an extension to \emph{non-metric} priors $J$ that
are of major importance for the success for our application scenario, we cannot
achieve this directly and have to go for a small detour.
\Ie the model has to be extended \emph{after} the discretisation into the
finite elementy (FEM) basis.
\end{comment}

We briefly explain why a non-metric model does not exist in the continuous
case without additional constraints on the functions spaces. % if we require lower semi-continuity of our energy \cite{maggi2012sets}.
%
Without additional constraints, one can always introduce a zero set, 
assigned to a label $j$, between any two
regions labeled $i$ and $k$, \ie a set with a Lebesque measure of $0$ in the
domain space.
Consequently the potentially higher transition cost for a non-metric label pair
$i,k$ compared to the sum of costs between $i,j$ and $j,k$
can always be avoided in the limit and non-metric energies are underestimated.
%implicitly becomes a metric.
%
%\todo{need some continuous equations here}.
%
%In practice, this is can become a serious problem, because the energy of the
%computed solution will be underestimated.
%in general by measuring the perimeter
%optimisation scheme will underestimate the energy of the computed solution.
%and the assigned energy will  not match.
%
In other words, let $S$ be a segmentation of $\Omega$ into regions $S^i$ and $S^k$,
labeled with $i$ and $k$ respectively, with costs that do not fulfill the triangle
inequality \wrt another label $j$.
Then one can find a sequence of segmentations $S^n:=\{S_i^n, S_j^n, S_k^n\}$
with $\displaystyle S=\lim_{n\to\infty} S^n$, \ie the label $j$ disappears in the limit case,
such that $\displaystyle \lim_{n\to\infty}\inf E(S^n) < E(S)$.
Hence, the metric property is a necessary condition for the lower
semi-continuity of our energy functional.
%On the other hand every metric regulariser implies the lsc. of our energy functional.
%
%
\begin{comment}
%labeled with $i,j,k$ respectively, such
% with non-metric transition costs, \ie the transition cost between
%$i,k$ does not fulfill the triangle inequality
%compared to $i,j$ and $j,k$
%is penalised
%
%that assign a higher penalty
%to label transitions $i,k$ compared to the sum of penalties between
%$i,j$ and $j,k$,
%one can find
we can find a sequence of segmentations
$S^n:=\{S_i^n, S_j^n, S_k^n\}$ with $S=\lim_{n\to\infty} S^n$
%
labeled with $i,j,k$ respectively, such
that $S_j^n$ disappears in the limit $n\rightarrow\infty$
for which $\displaystyle \lim_{n\to\infty}\inf E(S^n) < E(S)$.
%
%such that converges to the wrong solution
%triangle ineq implies lsc
\end{comment}
%
Methods that try to avoid this problem,
\eg by demanding Lipshitz continuity of the labeling functions
%and thus to guarantee convergence for non-metric priors
are an active research area,
\eg \cite{BreMas15}, but go beyond the scope of this work.

Any discretization of our domain will ultimately consist of only a finite number of 
elements of measurable ($>0$) volume. 
Thus, the label $j$ in the example above does not disappear %in the solution 
and the computed energy matches the solution. 
%
\begin{comment}
In the discrete setting, we have committed ourselves to a certain
tesselation of our domain and % we cannot find such a sequence;
the area assigned to a certain label cannot become a zero set. 
Thus the label $j$ does not disappear in the solution.
The computed energy matches the solution.
\end{comment}
%
%if one demands that each assignment
%\ie will the label will finally occur in the solution.
%
%However, this shows that our discrete solution will not converge to the
%continuous solution in the non-metric setting,
%
Our analysis implies, however, that a discrete solution in the non-metric
setting does not have a continuous counterpart and any investigation of the
limit case, \ie convergence analysis, 
after infinite refinements of the tesselation, is unreasonable. 
%
%It should be noted that, since our model is designed for the 
%non-metric relaxation of \cite{ZachHP14},  
%which does not posses a continuous counterpart 
%convergence to the continuous solution cannot be shown. 
%
%
%any convergence analysis to the continuous solution
%of our discrete energy is unreasonable.
%in the limit,
%our discrete solution will also converge to the wrong solution

%However, to perform infinite refinement steps appears unpractical and further more unreasonable

%  of the level of refinement of the tesselation of the domain.
%Thus, we start from the less general model of \cite{Strekalovskiy11}.

\subsubsection{Gradient in the Lagrange basis}
%
We repeat the statement from the paper, namely that 
we can compute a gradient in the P1 (Lagrange) basis that is 
constant per simplex $s$ and given by:
%
\begin{equation}\label{eq:gradient}
\nabla \phi_s = \sum_{v\in s} \phi_v J_{v}.
\end{equation}
%
Here, the coefficients $\phi_v\in \mathbb{R}$ and 
$J_{v}\in\mathbb{R}^d$ denote a vector, normal to the face $f_v$,
opposite to the node $v$ pointing inwards,
towards the center of the simplex with length $\frac{|f_v|}{|s|}$.
%
recall that $|f_v|$ denoted the area of the face $f_v$
and $|s|$ the volume of the simplex $s$ (\cf supplementary).

At first notice that the gradient of $\phi_t$ in (\ref{eq:gradient})
has to fulfill $\langle v_l-v_k; \nabla \phi_t \rangle = \phi_l-\phi_k$.
\Ie integration along the edge leads to the respective change
in $\phi_t$.  After collecting a sufficient number linear equations of this
form, one can directly solve the linear system. 
By noting that $J_{v}$ is orthogonal to all edges that do not involve 
vertex $v$ we arrive at \eqref{eq:gradient}.


\subsection{Data Term for Lagrange basis} % version of our
%
Although we could employ importance sampling to define the data cost 
$\rho^i_v$ and thus directly couple data term computation with the 
construction of $M$, we resort to a much simpler strategy. 
%
In \cite{HaneZCAP13} the data cost is evaluated on a regular grid, by
reprojecting grid vertices into the images, computing the data term and
adding the respective contribution to the grid location.
%
This corresponds to integrating the data cost within the respective
Voronoi-area of a vertex: the latter is proportional to the number of
regular samples falling within a Voronoi-cell, \ie have the respective
vertex as nearest neighbour.  Summing up the individual contribution
thus directly corresponds to integrating the data term within the
Voronoi region.
%
This procedure could easily be extended to importance sampling,
but it is not the computational bottleneck of the method, so we prefer
the simpler regular strategy.


%%%%%%%%%%%%%%%%%%%%%%%%%%%%%%%%%%%%%%%%%%%
\subsection{Raviart-Thomas Elements}
%
The Raviart-Thomas $\textrm{RT}^k(M)$ basis functions describe a
div-conforming polynomial basis of order $k\!+\!1$, here, on a
simplex mesh $M=\{F,V,S\}$ with vertices $v\in V, v\in\mathbb{R}^d$
faces $f\in F$ defined by $d$ vertices and
simplices $s\in S$, defined by $d+1$ vertices, that partition $\Omega$:
$\cup_k s_k=\Omega, s_l\cap s_k=f_{s,k}\in F$.
Here, two simplices share a single face.
%
\begin{align*}
&
RT^0(M) := \{ p:\Omega\rightarrow \mathbb{R}^d | p(x):=\sum_{s\in S} p_s(x) \textrm{ with }
\\ &
p_s(x):=c_s x + d_s, c_s\!\in\!\mathbb{R}, d_s\!\in \!\mathbb{R}^d,
\textrm{ if } x\!\in\! s \textrm{ and } 0 \textrm{ else},
\\
&
\textrm{and } p_s(x) \textrm{ is continuous for } x\in f_v(s) \textrm{ in direction } \nu_{f_v}
\}.
%
\end{align*}
%
Here we used $\nu_{f_v}$ to denote the normal of face $f_v$ of simplex s,
which, by convention, is located opposite to the vertex $v$.
%

We construct our linear basis with functions that are defined % \ie $k=0$
for each face $f_v$ opposite to a vertex $v$ in a simplex $s$
and can described in a local form as follows:
\begin{equation*}
p^{0}_{l,s,v}(x) := (x-v) |f_v|/|s| \quad \textrm{if}\; x\in s \;\textrm{and}\; 0 \;\textrm{else},
\end{equation*}
where we let $|f_v|$ denote the area of the face and $|s|$ $d$ times
the volume of the simplex.
We can read of $\textrm{div}(p^{0}_{s,v})=|f_v|/|s|$.
Let $\nu_{f_v}$ be the normal of face $f_v$, then the basis functions
fulfill
%
\begin{equation}\label{eq:property_RT}
\langle p^{0}_{s,u}(x), \nu_{f_v} \rangle := [u=v] \;\forall x\in f_v,
\end{equation}
where we make use of the Iverson bracket $[\cdot]$.
%
These basis functions make up the global function space by enforcing a
consistent orientation, for example we can distinguish for each face $f$
two simplices $s^+$ and $s^-$ analysing the scalar product of
the vector $\mathbf{1}$ and the normal $\nu^\pm_f$ of the shared face $f$
pointing outwards into each simplex.
Wlog we define $s^\pm$ via %the sign of
$\sign \langle \nu^\pm_f; \mathbf{1}\rangle$.
%s^\pm:= and $s^-$ accordingly.
The global basis functions per face $f_v$ opposite to
vertex $v$ are then given by:
\begin{equation}\label{eq:RT_global_basis}
p^{0}_{s^\pm,v} := \pm (x-v) |f_v|/|s^\pm| \quad \textrm{if}\; x\in s \;\textrm{and}\; 0 \;\textrm{else}.
\end{equation}
%
In each simplex a vector-field $\phi_s(x)\in\mathbb{R}^d$ is defined in
the following manner (with coefficients $\phi_v\in \mathbb{R}$):
\begin{equation*}
\phi_s(x) := \sum_{v\in s} \phi_v p^{0}_{s,v}.
\end{equation*}
%
By construction (\cf \eqref{eq:RT_global_basis}, \eqref{eq:property_RT}),
the vector-field has to be continuous along the face $x\in f_v$
normal direction $\nu_{f_v}$, \ie for neighbouring faces $\forall\phi_{s^\pm}$
we have: %s^\pm$
%orthogonal to the face
%
\begin{equation}\label{eq:RT-edgeSKP}
\langle \phi_{s^\pm}(x), \nu_{f_v} \rangle = \pm \langle x-v_\pm,\nu_{f_v}\rangle |f_v|/|s^\pm| \phi_{f_{v^\pm}} = \phi_{f_{v^\pm}}.
\end{equation}
%
Thus, our function is $\phi$ is a RT function iff for all neighbouring $s\pm$
faces we have $\phi_{f_{v^+}}=\phi_{f_{v^-}}$, or in other words basis
coefficients only exist for faces of the simplices.

Furthermore, the variables we are interested in are the labeling
functions $x^i$,
%
%which will be the dual multipliers of our objective in
%\eqref{eq:E-dual} after replacing the '$\min$' by its fenchel conjugate
%again
%(leading to the re-introduction of the indicator functions $x^i$
%and simplex constraints for these).
%The solution will be constant per simplex, \ie a piecewise constant labeling.
%Given a tesselation $S$ of $\Omega$, our
which are members of our test function space composed
of piecewise constant functions per simplex:
\begin{align*}
U^0(M):= \{ u:\Omega\rightarrow \mathbb{R} | &u(x):=\sum_{s\in S} u_s(x), \textrm{ with }
\\ &
u_s(x)=u_s \textrm{ if } x\!\in\! s \textrm{ and } 0 \textrm{ else}\}.
\end{align*}
%
With this choice, the defined basis is div-conforming:
%, the equivalence to the continuous case can be shown with the help of the divergence theorem:
%
\begin{align}\label{eq:discDiv}
& %_{|S}
\int_\Omega u(x) \div{}\phi(x) \dx = \sum_{s\in S}\int_S u_s \div\phi(x) \dx %\nonumber
=
\\
&
\sum_{s\in S}\int_{\partial S} \!\!\!\!u_s \langle \phi(x), \nu \rangle \dz
%\\
=
\sum_{\overset{v\in s}{s\in S}} u_s \phi_v |f_v|
=
\sum_{s\in S} u_s \div\phi(x) |s|.\nonumber
\end{align}
%p^{0}_{s,v}
Again, $\nu$ encodes the face normal $f_v$ of simplex $s$ pointing outwards.

Before we can utilise our new basis to discretise \eqref{eq:saddle} we need
proof that it is sufficient to enforce the constraints on our dual functions
$\phi$ in \eqref{eq:saddle} at the vertices of the simplex $s$.
%face midpoints $x_{f_v}$
to ensure the constraints are also valid for any point in the whole simplex.
%
The Wulff shapes are convex as are the linear inequalities in \eqref{eq:E-dual},
thus it is sufficient to proof that the vector field $\phi(x)$ at any
point $x\in s$ can be written as a convex combination:
%
\begin{equation*}%\label{eq:convexComb_edgemid}
\phi(z) = \sum_{f_v\in s} \alpha_{z,f_v} \phi(v), \textrm{with} \sum_{f_v\in s} \alpha_{z,f_v}=1.
\end{equation*}
%
After some algebra, it turns out that if $x=\alpha_i v_i$ then %$\phi(x) = (1-d\alpha_i) \phi(x_{f_{v_i}})$
$\alpha_{x,f_v}:=(1-d\cdot\alpha_i)$ encode this convex combination.

The same is true if the functions are evaluated at the vertex positions:
\begin{equation}\label{eq:convexComb}
\phi(x) = \sum_{v\in s} \alpha_{v} \phi(v), \textrm{with} \sum_{v\in s} \alpha_v=1.
\end{equation}
%
This has the additional advantage that one face in the summation can be
ignored and evaluation at a point can be written as a matrix
multiplication with an invertible matrix
(from relevant basis coefficients to value at the point and back).
This is useful in the linear constraint set.

In a simplex $s$ the RT function $\phi_s(x) := \sum_{v\in s} \phi_v p^{0}_{s,v}(x)$
evaluated at the face midpoint $x_{f_v}=1/d\sum_{w \in s, w\neq v}w$ becomes:
\begin{equation*}
\phi_s(x_{f_v}) = - \phi_v\frac{|f_v|}{|s|} v -\!\!\!\!\! \sum_{w\in s, w\neq v} \!\!\!\!\!\frac{w}{d}(\phi_w\frac{|f_w|}{|s|} -\!\!\!\! \sum_{u\in s, u\neq w}\!\!\! \phi_u\frac{|f_u|}{|s|}).
\end{equation*}

If we utilise the values at the vertices we receive a seemingly simpler but
certainly more compact representation. To compute $\phi(v)$ for some vertex $v$
of the simplex $s$, we can compose a linear map:
\begin{align}\label{eq:project_matrix}
  \phi(v) = \sum_{v_i\in s, v_i\neq v} (v-v_i) \frac{|f_{v_i}|}{|s|} \phi_{v_i},
\end{align}
%
which can also be assembled in matrix form $\phi_s(v) = M_{s,v} \phi_{s,v}$,
with an invertible matrix $M_{s,v}$.
The columns are a weighted combination of the edges towards the
vertex $v$ to be evaluated \eqref{eq:project_matrix}.
Apparently we can compute all but one coefficient from the value at one
vertex already.
%


\begin{comment}
\begin{comment}
% too complex for now.

\subsection{Raviart-Thomas Elements}
%
The Raviart-Thomas $\textrm{RT}^k(M)$ basis functions describe a
div-conforming polynomial basis of order $k\!+\!1$, here, on a
simplex mesh $M=\{F,V,S\}$ with vertices $v\in V, v\in\mathbb{R}^d$
faces $f\in F$ defined by $d$ vertices and
simplices $s\in S$, defined by $d+1$ vertices, that partition $\Omega$:
$\cup_k s_k=\Omega, s_l\cap s_k=f_{s,k}\in F$.
Here, two simplices share a single face.
%
\begin{align*}
&
RT^0(M) := \{ p:\Omega\rightarrow \mathbb{R}^d | p(x):=\sum_{s\in S} p_s(x) \textrm{ with }
\\ &
p_s(x):=c_s x + d_s, c_s\!\in\!\mathbb{R}, d_s\!\in \!\mathbb{R}^d,
\textrm{ if } x\!\in\! s \textrm{ and } 0 \textrm{ else},
\\
&
\textrm{and } p_s(x) \textrm{ is continuous for } x\in f_v(s) \textrm{ in direction } \nu_{f_v}
\}.
%
\end{align*}
%
Here we used $\nu_{f_v}$ to denote the normal of face $f_v$ of simplex s,
which, by convention, is located opposite to the vertex $v$.
%

We construct our linear basis with functions that are defined % \ie $k=0$
for each face $f_v$ opposite to a vertex $v$ in a simplex $s$
and can described in a local form as follows:
\begin{equation*}
p^{0}_{l,s,v}(x) := (x-v) |f_v|/|s| \quad \textrm{if}\; x\in s \;\textrm{and}\; 0 \;\textrm{else},
\end{equation*}
where we let $|f_v|$ denote the area of the face and $|s|$ $d$ times
the volume of the simplex.
We can read of $\textrm{div}(p^{0}_{s,v})=|f_v|/|s|$.
Let $\nu_{f_v}$ be the normal of face $f_v$, then the basis functions
fulfill
%
\begin{equation}\label{eq:property_RT}
\langle p^{0}_{s,u}(x), \nu_{f_v} \rangle := [u=v] \;\forall x\in f_v,
\end{equation}
where we make use of the Iverson bracket $[\cdot]$.
%
These basis functions make up the global function space by enforcing a
consistent orientation, for example we can distinguish for each face $f$
two simplices $s^+$ and $s^-$ analysing the scalar product of
the vector $\mathbf{1}$ and the normal $\nu^\pm_f$ of the shared face $f$
pointing outwards into each simplex.
Wlog we define $s^\pm$ via %the sign of
$\sign \langle \nu^\pm_f; \mathbf{1}\rangle$.
%s^\pm:= and $s^-$ accordingly.
The global basis functions per face $f_v$ opposite to
vertex $v$ are then given by:
\begin{equation}\label{eq:RT_global_basis}
p^{0}_{s^\pm,v} := \pm (x-v) |f_v|/|s^\pm| \quad \textrm{if}\; x\in s \;\textrm{and}\; 0 \;\textrm{else}.
\end{equation}
%
In each simplex a vector-field $\phi_s(x)\in\mathbb{R}^d$ is defined in
the following manner (with coefficients $\phi_v\in \mathbb{R}$):
\begin{equation*}
\phi_s(x) := \sum_{v\in s} \phi_v p^{0}_{s,v}.
\end{equation*}
%
By construction (\cf \eqref{eq:RT_global_basis}, \eqref{eq:property_RT}),
the vector-field has to be continuous along the face $x\in f_v$
normal direction $\nu_{f_v}$, \ie for neighbouring faces $\forall\phi_{s^\pm}$
we have: %s^\pm$
%orthogonal to the face
%
\begin{equation}\label{eq:RT-edgeSKP}
\langle \phi_{s^\pm}(x), \nu_{f_v} \rangle = \pm \langle x-v_\pm,\nu_{f_v}\rangle |f_v|/|s^\pm| \phi_{f_{v^\pm}} = \phi_{f_{v^\pm}}.
\end{equation}
%
Thus, our function is $\phi$ is a RT function iff for all neighbouring $s\pm$
faces we have $\phi_{f_{v^+}}=\phi_{f_{v^-}}$, or in other words basis
coefficients only exist for faces of the simplices.

Furthermore, the variables we are interested in are the labeling
functions $x^i$,
%
%which will be the dual multipliers of our objective in
%\eqref{eq:E-dual} after replacing the '$\min$' by its fenchel conjugate
%again
%(leading to the re-introduction of the indicator functions $x^i$
%and simplex constraints for these).
%The solution will be constant per simplex, \ie a piecewise constant labeling.
%Given a tesselation $S$ of $\Omega$, our
which are members of our test function space composed
of piecewise constant functions per simplex:
\begin{align*}
U^0(M):= \{ u:\Omega\rightarrow \mathbb{R} | &u(x):=\sum_{s\in S} u_s(x), \textrm{ with }
\\ &
u_s(x)=u_s \textrm{ if } x\!\in\! s \textrm{ and } 0 \textrm{ else}\}.
\end{align*}
%
With this choice, the defined basis is div-conforming:
%, the equivalence to the continuous case can be shown with the help of the divergence theorem:
%
\begin{align}\label{eq:discDiv}
& %_{|S}
\int_\Omega u(x) \div{}\phi(x) \dx = \sum_{s\in S}\int_S u_s \div\phi(x) \dx %\nonumber
=
\\
&
\sum_{s\in S}\int_{\partial S} \!\!\!\!u_s \langle \phi(x), \nu \rangle \dz
%\\
=
\sum_{\overset{v\in s}{s\in S}} u_s \phi_v |f_v|
=
\sum_{s\in S} u_s \div\phi(x) |s|.\nonumber
\end{align}
%p^{0}_{s,v}
Again, $\nu$ encodes the face normal $f_v$ of simplex $s$ pointing outwards.

Before we can utilise our new basis to discretise \eqref{eq:saddle} we need
proof that it is sufficient to enforce the constraints on our dual functions
$\phi$ in \eqref{eq:saddle} at the vertices of the simplex $s$.
%face midpoints $x_{f_v}$
to ensure the constraints are also valid for any point in the whole simplex.
%
The Wulff shapes are convex as are the linear inequalities in \eqref{eq:E-dual},
thus it is sufficient to proof that the vector field $\phi(x)$ at any
point $x\in s$ can be written as a convex combination:
%
\begin{equation*}%\label{eq:convexComb_edgemid}
\phi(z) = \sum_{f_v\in s} \alpha_{z,f_v} \phi(v), \textrm{with} \sum_{f_v\in s} \alpha_{z,f_v}=1.
\end{equation*}
%
After some algebra, it turns out that if $x=\alpha_i v_i$ then %$\phi(x) = (1-d\alpha_i) \phi(x_{f_{v_i}})$
$\alpha_{x,f_v}:=(1-d\cdot\alpha_i)$ encode this convex combination.

The same is true if the functions are evaluated at the vertex positions:
\begin{equation}\label{eq:convexComb}
\phi(x) = \sum_{v\in s} \alpha_{v} \phi(v), \textrm{with} \sum_{v\in s} \alpha_v=1.
\end{equation}
%
This has the additional advantage that one face in the summation can be
ignored and evaluation at a point can be written as a matrix
multiplication with an invertible matrix
(from relevant basis coefficients to value at the point and back).
This is useful in the linear constraint set.

In a simplex $s$ the RT function $\phi_s(x) := \sum_{v\in s} \phi_v p^{0}_{s,v}(x)$
evaluated at the face midpoint $x_{f_v}=1/d\sum_{w \in s, w\neq v}w$ becomes:
\begin{equation*}
\phi_s(x_{f_v}) = - \phi_v\frac{|f_v|}{|s|} v -\!\!\!\!\! \sum_{w\in s, w\neq v} \!\!\!\!\!\frac{w}{d}(\phi_w\frac{|f_w|}{|s|} -\!\!\!\! \sum_{u\in s, u\neq w}\!\!\! \phi_u\frac{|f_u|}{|s|}).
\end{equation*}

If we utilise the values at the vertices we receive a seemingly simpler but
certainly more compact representation. To compute $\phi(v)$ for some vertex $v$
of the simplex $s$, we can compose a linear map:
\begin{align}\label{eq:project_matrix}
  \phi(v) = \sum_{v_i\in s, v_i\neq v} (v-v_i) \frac{|f_{v_i}|}{|s|} \phi_{v_i},
\end{align}
%
which can also be assembled in matrix form $\phi_s(v) = M_{s,v} \phi_{s,v}$,
with an invertible matrix $M_{s,v}$.
The columns are a weighted combination of the edges towards the
vertex $v$ to be evaluated \eqref{eq:project_matrix}.
Apparently we can compute all but one coefficient from the value at one
vertex already.
%
%
Instead of repeating the complete derivation for the P1 basis of piecewise
linear functions on our simplex partition we follow an alternative route,
which allows for additional insights into the original grid based formulation
of \cite{HaneZCAP13,ZachHP14} and is pleasantly visual.

Dual graph for grid follows P1

\end{comment}
